# Supplementary material for: Discrete MMSE Precoding for Multiuser MIMO Systems with PSK Modulation
Source: arXiv:2105.11555 source file (2021-05-24)
Supplement: Supplementary file 1 [file conditios_zero_mean.tex]

\subsection{Conditions for a zero mean error term}
\label{subsec:conditions}

In this section we derive the conditions that need be fulfilled for $\text{E}\chav{\epsilon_k[t]|s}=0$. Following $\text{E}\chav{\epsilon_k[t]|s}$ is expanded and equated to zero
\vspace{0.2em}
\begin{align}
&\text{E}\chav{\epsilon_k[t]|s}=\text{E}\chav{z_k[t]-h_{eff}^k\  s-w_k[t]|s}\notag\\
&=\text{E}\chav{\boldsymbol{h}_k\ \boldsymbol{x}(\boldsymbol{s})|s}-h_{eff}^k \ s \notag \\
&=\boldsymbol{h}_k\ \text{E}\chav{ \boldsymbol{x}(\boldsymbol{s})|s}-\frac{s}{\sigma_s^2}\text{E}\chav{s_k^*(\boldsymbol{s}) \boldsymbol{h}_k\ \boldsymbol{x}(\boldsymbol{s})}\notag \\
&=\frac{1}{\alpha_s^{(K-1)}}\boldsymbol{h}_k \pc{\displaystyle \sum_{\boldsymbol{s}\in \mathcal{D}} \boldsymbol{x}(\boldsymbol{s})-
{\frac{s}{\sigma_s^2 \alpha_s}}\sum_{\boldsymbol{s}\in \mathcal{S}^K} \ s^*_k(\boldsymbol{s}) \boldsymbol{x}(\boldsymbol{s})}=0.\notag
\end{align}
The previous equation is equal to zero when the following holds
\begin{align}
&\displaystyle \sum_{\boldsymbol{s}\in \mathcal{D}} \boldsymbol{x} (\boldsymbol{s})=
{\frac{s\ }{\sigma_s^2 \ \alpha_s}}\sum_{\boldsymbol{s}\in \mathcal{S}^K} \ s^*_k(\boldsymbol{s})\ \boldsymbol{x} (\boldsymbol{s})\notag\\
\label{eq:appendix1}
&\displaystyle \sum_{\bar{\boldsymbol{s}}\in \mathcal{S}^{K-1}}\boldsymbol{x}\pc{ {s},  \bar{\boldsymbol{s}}}=
{\frac{{s}}{\sigma_s^2 \ \alpha_s}} \sum_{{\tilde{s}}\in \mathcal{S}}\ \ \sum_{\boldsymbol{\bar{s}}\in \mathcal{S}^{K-1}}\pc{\tilde{s}}^{*} \boldsymbol{x}\pc{{\tilde{s},\bar{\boldsymbol{s}}}}.
\end{align}
By defining $\tilde{s}=s\ e^{j \Delta \phi_{s \tilde{s}}}$, equation \eqref{eq:appendix1} can be rewritten as
\begin{align}
&\displaystyle \sum_{\bar{\boldsymbol{s}}\in \mathcal{S}^{K-1}}\boldsymbol{x}\pc{ {s},  \bar{\boldsymbol{s}}}=\notag\\
&{\frac{{s}}{\sigma_s^2 \ \alpha_s}} \sum_{{\tilde{s}}\in \mathcal{S}}\ \ \sum_{\boldsymbol{\bar{s}}\in \mathcal{S}^{K-1}} \pc{s\ e^{j \Delta \phi_{s \tilde{s}}}}^* \boldsymbol{x}\pc{{{s\ e^{j \Delta \phi_{s \tilde{s}}}}},\bar{\boldsymbol{s}}}\notag.
\end{align}
Further expanding the symbol vector by multiplication with $e^{j \Delta \phi_{s \tilde{s}}} e^{-j \Delta \phi_{s \tilde{s}}}$ yields
\begin{align}
&\displaystyle \sum_{\bar{\boldsymbol{s}}\in \mathcal{S}^{K-1}}\boldsymbol{x}\pc{ {s},  \bar{\boldsymbol{s}}}=\notag\\
&{\frac{{s}}{\sigma_s^2 \ \alpha_s}} \sum_{{\tilde{s}}\in \mathcal{S}}\sum_{\boldsymbol{\bar{s}}\in \mathcal{S}^{K-1}} \pc{s e^{j \Delta \phi_{s \tilde{s}}}}^* \boldsymbol{x}\pc{{{s e^{j \Delta \phi_{s \tilde{s}}}}},\bar{\boldsymbol{s}} e^{j \Delta \phi_{s \tilde{s}}}  e^{-j \Delta \phi_{s \tilde{s}}}}\notag.
 \end{align}
Moreover, it is considered that the precoding process is circular symmetric meaning that given an angle $\phi = \frac{\pi \pc{2 i+1}}{\alpha_x},\ i=1...\alpha_x $, the precoder vector $\boldsymbol{x}\pc{\boldsymbol{s}}$ has the property $\boldsymbol{x}\pc{\boldsymbol{s} \ e^{\ j \phi}}=\boldsymbol{x}\pc{\boldsymbol{s}} e^{\ j \phi}$. Note that, the angle $\Delta \phi_{s \tilde{s}}$ has the form $\Delta \phi_{s \tilde{s}} = \frac{\pi \pc{2 i+1}}{\alpha_s},\ i=1...\alpha_s$. If $\alpha_x=\alpha_s$ is chosen, the following holds
\begin{align}
\label{eq:appendix2}
\displaystyle \sum_{\bar{\boldsymbol{s}}\in \mathcal{S}^{K-1}}&\boldsymbol{x}\pc{ {s},  \bar{\boldsymbol{s}}}=\notag\\
&{\frac{{s}}{\sigma_s^2 \alpha_s}} \sum_{{\tilde{s}}\in \mathcal{S}}\sum_{\boldsymbol{\bar{s}}\in \mathcal{S}^{K-1}} \pc{s \ e^{j \Delta \phi_{s \tilde{s}}}}^* e^{j \Delta \phi_{s \tilde{s}}} \boldsymbol{x}\pc{s,\bar{\boldsymbol{s}} \ e^{-j \Delta \phi_{s \tilde{s}}}}.
\end{align}
Considering that for PSK symbols, $\sigma_s^2=\PM{s}^2 \ \forall  \ s\in \mathcal{S}^K$ equation \eqref{eq:appendix2} can be rewritten as
\begin{align}
&\displaystyle \sum_{\bar{\boldsymbol{s}}\in \mathcal{S}^{K-1}}\boldsymbol{x}\pc{ {s},  \bar{\boldsymbol{s}}}=
\pc{\frac{{1}}{\alpha_s}} \sum_{{\tilde{s}}\in \mathcal{S}}\ \ \sum_{\boldsymbol{\bar{s}}\in \mathcal{S}^{K-1}}   \boldsymbol{x}\pc{s,\bar{\boldsymbol{s}} \ e^{-j \Delta \phi_{s \tilde{s}}}}\notag\\
&\displaystyle \sum_{\bar{\boldsymbol{s}}\in \mathcal{S}^{K-1}}\boldsymbol{x}\pc{ {s},  \bar{\boldsymbol{s}}}=
\pc{\frac{{1}}{\alpha_s}} \sum_{{\tilde{s}}\in \mathcal{S}}\ \ \sum_{\boldsymbol{\bar{s}}\in \mathcal{R}}   \boldsymbol{x}\pc{s,\bar{\boldsymbol{s}}}\notag,
\end{align}
where $\mathcal{R}$ is the set $\mathcal{S}^{K-1}$ rotated by $\Delta \phi_{s \tilde{s}}$. Note that since $\alpha_x=\alpha_s$, the rotation produces the same set meaning that $\mathcal{R}=\mathcal{S}^{K-1}$.
 Then, 
 \begin{align}
&\displaystyle \sum_{\bar{\boldsymbol{s}}\in \mathcal{S}^{K-1}}\boldsymbol{x}\pc{ {s},  \bar{\boldsymbol{s}}}=
\pc{\frac{{1}}{\alpha_s}} \sum_{{\tilde{s}}\in \mathcal{S}}\ \ \sum_{\boldsymbol{\bar{s}}\in \mathcal{S}^{K-1}}   \boldsymbol{x}\pc{s,\bar{\boldsymbol{s}}}.\notag
\end{align}
Since $\boldsymbol{x}\pc{s,\bar{\boldsymbol{s}}}$ does not depend on $\tilde{s}$ and the cardinality of the set $\mathcal{S}$ is $\alpha_s$ the equality holds. Thus equation \eqref{eq:appendix1} holds with equality.
